# Supplementary material for: Anomalous Behavior of Magnetic Susceptibility Obtained by Quench Experiments in Isolated Quantum Systems
Source: arXiv:1911.02456 source file (2020-03-14)
Supplement: Supplementary file 1 [file SupplementalMaterial_2020Mar06.pdf]

# Anomalous Behavior of Magnetic Susceptibility Obtained by Quench Experiments in Isolated Quantum Systems: *Supplemental Material*

Yuuya Chiba* and Akira Shimizu†
*Komaba Institute for Science, The University of Tokyo, 3-8-1 Komaba, Meguro, Tokyo 153-8902, Japan and Department of Basic Science, The University of Tokyo, 3-8-1 Komaba, Meguro, Tokyo 153-8902, Japan*

Kenichi Asano‡
*Center for Education in Liberal Arts and Sciences, Osaka University, Toyonaka, Osaka 560-0043, Japan*
(Dated: March 14, 2020)

## A. Quench susceptibility

We deal with a quantum spin system on a $d$-dimensional hypercubic lattice $\Omega_N$ with linear size $L$ and $N = |\Omega_N| = L^d$ spins centered at $\boldsymbol{r} = \boldsymbol{0}$. The unit of length is taken as the lattice constant. We consider a quantum quench process where the weak additional field $\Delta h(\boldsymbol{r})$, with wave number $\boldsymbol{k}$ and magnitude $\Delta h_{\boldsymbol{k}}$, is applied suddenly at $t = 0$ and after that the expectation value of $\hat{\sigma}^z_{\boldsymbol{r}}$ evolves in time as

$$\langle \hat{\sigma}^z_{\boldsymbol{r}} \rangle^{\rm qch}(t) = \langle \hat{\sigma}^z_{\boldsymbol{r}} \rangle_{\rm ini} + \sum_{\boldsymbol{r}' \in \Omega_N} \phi^{\rm qch}_N(\boldsymbol{r} - \boldsymbol{r}'; t) \Delta h(\boldsymbol{r}') + \mathcal{O}(\Delta h^2_{\boldsymbol{k}}), \tag{S1}$$

where $\langle \bullet \rangle_{\rm ini} = {\rm Tr}[\hat{\rho}_{\rm ini} \bullet]$. Here, $\phi^{\rm qch}_N(\boldsymbol{r}; t) = \beta \langle \delta\hat{\sigma}^z_{\boldsymbol{0}}; \delta\hat{\sigma}^z_{\boldsymbol{r}} \rangle_{\rm ini} - \beta \langle \delta\hat{\sigma}^z_{\boldsymbol{0}}; \delta\hat{\sigma}^z_{\boldsymbol{r}}(t) \rangle_{\rm ini}$ is a periodic function of $\boldsymbol{r}$ with period $L$, where $\hat{X}(t) = e^{i\hat{H}(h)t} \hat{X} e^{-i\hat{H}(h)t}$ is the Heisenberg operator and $\langle \hat{X}; \hat{Y} \rangle_{\rm ini} = \frac{1}{\beta} \int_0^\beta {\rm d}u \, \langle e^{u\hat{H}(h)} \hat{X}^\dagger e^{-u\hat{H}(h)} \hat{Y} \rangle_{\rm ini}$ is the canonical correlation. Then, the response of $\hat{m}_{\boldsymbol{k}}$ at time $t$ reads $\Delta\langle \hat{m}_{\boldsymbol{k}} \rangle^{\rm qch}(t) = \langle \hat{m}_{\boldsymbol{k}} \rangle^{\rm qch}(t) - \langle \hat{m}_{\boldsymbol{k}} \rangle_{\rm ini} = \chi^{\rm qch}_N(\boldsymbol{k}; t) \Delta h_{\boldsymbol{k}} + \mathcal{O}(\Delta h^2_{\boldsymbol{k}})$, where

$$\chi^{\rm qch}_N(\boldsymbol{k}; t) = \sum_{\boldsymbol{r} \in \Omega_N} e^{-i\boldsymbol{k}\cdot\boldsymbol{r}} \phi^{\rm qch}_N(\boldsymbol{r}; t) = \beta N \langle \delta\hat{m}_{\boldsymbol{k}}; \delta\hat{m}_{\boldsymbol{k}} \rangle_{\rm ini} - \beta N \langle \delta\hat{m}_{\boldsymbol{k}}; \delta\hat{m}_{\boldsymbol{k}}(t) \rangle_{\rm ini}. \tag{S2}$$

Since we are only interested in the relaxed value of $\Delta\langle \hat{m}_{\boldsymbol{k}} \rangle^{\rm qch}(t)$, we define the quench susceptibility $\chi^{\rm qch}_N(\boldsymbol{k})$ as the long time average of $\chi^{\rm qch}_N(\boldsymbol{k}; t)$,

$$\chi^{\rm qch}_N(\boldsymbol{k}) = \lim_{\mathcal{T} \to \infty} \overline{\chi^{\rm qch}_N(\boldsymbol{k}; t)}^{\mathcal{T}} = \beta N \langle \delta\hat{m}_{\boldsymbol{k}}; \delta\hat{m}_{\boldsymbol{k}} \rangle_{\rm ini} - \beta N \langle \delta\hat{m}^0_{\boldsymbol{k}}; \delta\hat{m}^0_{\boldsymbol{k}} \rangle_{\rm ini}. \tag{S3}$$

Here the energy diagonal part of an operator $\hat{X}$ is given as $\hat{X}^0 = \lim_{\mathcal{T} \to \infty} \overline{\hat{X}(t)}^{\mathcal{T}} = \sum_{\nu,\nu'} \delta_{E_\nu, E_{\nu'}} |\nu\rangle \langle \nu | \hat{X} | \nu' \rangle \langle \nu' |$.

Figures S1(a) and S1(b) show the time dependence of $\chi^{\rm qch}_N(0; t)$ and $\chi^{\rm qch}_N(\pi/2; t)$ in 1D $XYZ$ model, respectively. For $t \gtrsim 5$, i.e., after the transient regime, $\chi^{\rm qch}_N(k; t)$ fluctuates in time around the quench susceptibility $\chi^{\rm qch}_N(k)$, which is shown by the solid line. When the system size $N$ is increased as 8, 12 and 16, this time fluctuation gets small. Therefore, if $\chi^{\rm qch}_N(k; t)$ is measured after the transient regime, the measured value of $\chi^{\rm qch}_N(k; t)$ will be close to $\chi^{\rm qch}_N(k)$.

In the definition of $\chi^{\rm qch}_N(\boldsymbol{k})$, $N$ is kept finite until the two limits $\Delta h_{\boldsymbol{k}} \to 0$ and $\mathcal{T} \to \infty$ are taken. This is reasonable in the sense that experiments on isolated quantum systems are performed only for finite $N$, such as $N \simeq 30$ [1].

## B. Thermodynamic susceptibilities

We consider the isothermal quasistatic process in which the weak additional field is applied gradually and the final state of the system is the canonical Gibbs one, $\hat{\rho}^T_{\rm fin} \propto \exp\big(-\beta(\hat{H}(h) - \sum_{\boldsymbol{r} \in \Omega_N} \hat{\sigma}^z_{\boldsymbol{r}} \Delta h(\boldsymbol{r}))\big)$, with the same inverse

* chiba@as.c.u-tokyo.ac.jp
† shmz@as.c.u-tokyo.ac.jp
‡ asano@celas.osaka-u.ac.jp

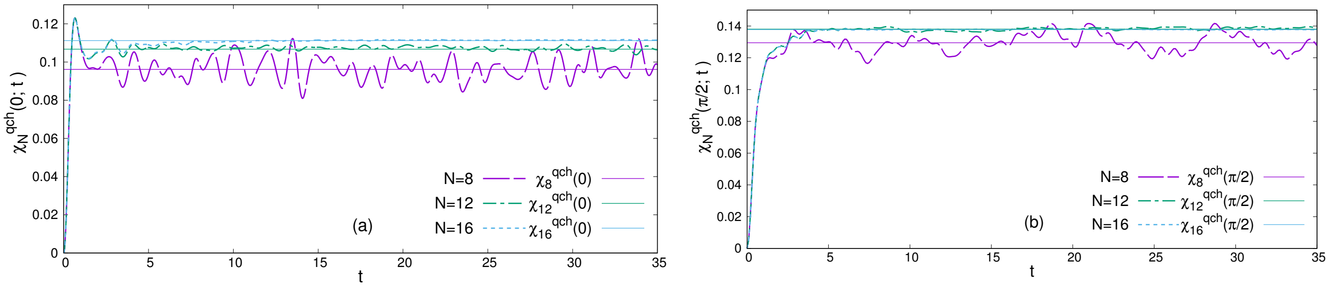


FIG. S1. Time dependence of (a) $\chi_N^{\mathrm{qch}}(0;t)$ and (b) $\chi_N^{\mathrm{qch}}(\pi/2;t)$ in $XYZ$ model, with the parameters, $J_x+J_y=0.6$, $J_x-J_y=1.2$, $J_z=1.0$, $h=0.8$, and $\beta=0.15$. We take $N=8,12,16$. The solid lines in (a) and (b) show $\chi_N^{\mathrm{qch}}(0)$ and $\chi_N^{\mathrm{qch}}(\pi/2)$ for each $N$, respectively. As the system size $N$ is increased, the time fluctuation of $\chi_N^{\mathrm{qch}}(k;t)$ from its time average $\chi_N^{\mathrm{qch}}(k)$ gets small in both (a) and (b).

temperature as the initial one. Then, the expectation value of $\hat{\sigma}_{\boldsymbol{r}}^z$ changes by

$$\Delta\langle\hat{\sigma}_{\boldsymbol{r}}^z\rangle^T = \mathrm{Tr}[\hat{\rho}_{\mathrm{fin}}^T\hat{\sigma}_{\boldsymbol{r}}^z] - \langle\hat{\sigma}_{\boldsymbol{r}}^z\rangle_{\mathrm{ini}} = \sum_{\boldsymbol{r}'\in\Omega_N}\phi_N^T(\boldsymbol{r}-\boldsymbol{r}')\Delta h(\boldsymbol{r}') + \mathcal{O}(\Delta h_{\boldsymbol{k}}^2), \tag{S4}$$

where $\phi_N^T(\boldsymbol{r}) = \beta\langle\delta\hat{\sigma}_{\boldsymbol{0}}^z;\delta\hat{\sigma}_{\boldsymbol{r}}^z\rangle_{\mathrm{ini}}$ is defined as a periodic function of $\boldsymbol{r}$ in the same way as $\phi_N^{\mathrm{qch}}(\boldsymbol{r};t)$. From Eq. (S4), the response of $\hat{m}_{\boldsymbol{k}}$ is given as $\Delta\langle\hat{m}_{\boldsymbol{k}}\rangle^T = \mathrm{Tr}[\hat{\rho}_{\mathrm{fin}}^T\hat{m}_{\boldsymbol{k}}] - \langle\hat{m}_{\boldsymbol{k}}\rangle_{\mathrm{ini}} = \chi_N^T(\boldsymbol{k})\Delta h_{\boldsymbol{k}} + \mathcal{O}(\Delta h_{\boldsymbol{k}}^2)$, where

$$\chi_N^T(\boldsymbol{k}) = \sum_{\boldsymbol{r}\in\Omega_N} e^{-i\boldsymbol{k}\cdot\boldsymbol{r}}\phi_N^T(\boldsymbol{r}) = \beta N\langle\delta\hat{m}_{\boldsymbol{k}};\delta\hat{m}_{\boldsymbol{k}}\rangle_{\mathrm{ini}} \tag{S5}$$

is the isothermal susceptibility.

We also consider the adiabatic quasistatic process in which the weak additional field is applied gradually and the final state of the system is the canonical Gibbs one $\hat{\rho}_{\mathrm{fin}}^S \propto \exp\left(-\beta_{\mathrm{fin}}^S(\hat{H}(h) - \sum_{\boldsymbol{r}\in\Omega_N}\hat{\sigma}_{\boldsymbol{r}}^z\Delta h(\boldsymbol{r}))\right)$ with the same entropy as the initial one, $-\mathrm{Tr}[\hat{\rho}_{\mathrm{fin}}^S\log\hat{\rho}_{\mathrm{fin}}^S]/N = -\mathrm{Tr}[\hat{\rho}_{\mathrm{ini}}\log\hat{\rho}_{\mathrm{ini}}]/N$. From this condition, the final inverse temperature $\beta_{\mathrm{fin}}^S$ is determined as

$$\beta_{\mathrm{fin}}^S = \beta + \sum_{\boldsymbol{r}\in\Omega_N}\beta\frac{\langle\delta\hat{H}(h)\ \delta\hat{\sigma}_{\boldsymbol{r}}^z\rangle_{\mathrm{ini}}}{\langle\delta\hat{H}(h)^2\rangle_{\mathrm{ini}}}\Delta h(\boldsymbol{r}) + \mathcal{O}(\Delta h_{\boldsymbol{k}}^2). \tag{S6}$$

The change of the expectation value of $\hat{\sigma}_{\boldsymbol{r}}^z$, $\Delta\langle\hat{\sigma}_{\boldsymbol{r}}^z\rangle^S = \mathrm{Tr}[\hat{\rho}_{\mathrm{fin}}^S\hat{\sigma}_{\boldsymbol{r}}^z] - \langle\hat{\sigma}_{\boldsymbol{r}}^z\rangle_{\mathrm{ini}}$, is given as

$$\Delta\langle\hat{\sigma}_{\boldsymbol{r}}^z\rangle^S = \Delta\langle\hat{\sigma}_{\boldsymbol{r}}^z\rangle^T - (\beta_{\mathrm{fin}}^S-\beta)\langle\delta\hat{H}(h)\ \delta\hat{\sigma}_{\boldsymbol{r}}^z\rangle_{\mathrm{ini}} + \mathcal{O}(\Delta h_{\boldsymbol{k}}^2) = \sum_{\boldsymbol{r}'\in\Omega_N}\phi_N^S(\boldsymbol{r}-\boldsymbol{r}')\Delta h(\boldsymbol{r}') + \mathcal{O}(\Delta h_{\boldsymbol{k}}^2), \tag{S7}$$

where

$$\phi_N^S(\boldsymbol{r}) = \phi_N^T(\boldsymbol{r}) - \beta\frac{\langle\delta\hat{H}(h)\ \delta\hat{\sigma}_{\boldsymbol{0}}^z\rangle_{\mathrm{ini}}^2}{\langle\delta\hat{H}(h)^2\rangle_{\mathrm{ini}}}. \tag{S8}$$

Then, the response of $\hat{m}_{\boldsymbol{k}}$ is also given as $\Delta\langle\hat{m}_{\boldsymbol{k}}\rangle^S = \mathrm{Tr}[\hat{\rho}_{\mathrm{fin}}^S\hat{m}_{\boldsymbol{k}}] - \langle\hat{m}_{\boldsymbol{k}}\rangle_{\mathrm{ini}} = \chi_N^S(\boldsymbol{k})\Delta h_{\boldsymbol{k}} + \mathcal{O}(\Delta h_{\boldsymbol{k}}^2)$, where

$$\chi_N^S(\boldsymbol{k}) = \sum_{\boldsymbol{r}\in\Omega_N} e^{-i\boldsymbol{k}\cdot\boldsymbol{r}}\phi_N^S(\boldsymbol{r}) = \chi_N^T(\boldsymbol{k}) - \beta N\frac{|\langle\delta\hat{H}(h)\ \delta\hat{m}_{\boldsymbol{k}}\rangle_{\mathrm{ini}}|^2}{\langle\delta\hat{H}(h)^2\rangle_{\mathrm{ini}}} \tag{S9}$$

is the adiabatic susceptibility.

### C. Relations between the susceptibilities

From Eq. (S9), we have $\chi_N^S(\boldsymbol{k}) = \chi_N^T(\boldsymbol{k}) - \frac{T}{c_h}\left|(\partial m_{\boldsymbol{k}}/\partial T)_h\right|^2$, where $c_h = \beta^2\langle\delta\hat{H}(h)^2\rangle_{\mathrm{ini}}/N$ is the specific heat at constant magnetic field and $(\partial m_{\boldsymbol{k}}/\partial T)_h = -\beta^2\langle\delta\hat{H}(h)\delta\hat{m}_{\boldsymbol{k}}\rangle_{\mathrm{ini}}$. In contrast to $\boldsymbol{k}=\boldsymbol{0}$ component, $(\partial m_{\boldsymbol{k}}/\partial T)_h = 0$ hold for all $\boldsymbol{k}\neq\boldsymbol{0}$ because of the translation invariance of $\hat{H}(h)$, yielding

$$\chi_N^S(\boldsymbol{k}) = \chi_N^T(\boldsymbol{k}) \quad \text{for all } \boldsymbol{k}\neq\boldsymbol{0}. \tag{S10}$$

Comparing Eqs. (S3) and (S9), we have

$$\chi_N^S(\mathbf{0}) - \chi_N^{\rm qch}(\mathbf{0}) = \beta N \langle \delta\hat{m}^0_{\boldsymbol{k}=\mathbf{0}}; \delta\hat{m}^0_{\boldsymbol{k}=\mathbf{0}}\rangle_{\rm ini} - \beta N \frac{|\langle \delta\hat{H}(h)\ \delta\hat{m}_{\boldsymbol{k}=\mathbf{0}}\rangle_{\rm ini}|^2}{\langle \delta\hat{H}(h)^2\rangle_{\rm ini}} \tag{S11}$$

$$= \beta N \Big(\sum_\nu \frac{e^{-\beta E_\nu}}{Z} \langle\nu|\delta\hat{\sigma}^z_{\mathbf{0}}|\nu\rangle^2\Big) - \beta N \Big(\sum_\nu \frac{e^{-\beta E_\nu}}{Z} \delta E_\nu \langle\nu|\delta\hat{\sigma}^z_{\mathbf{0}}|\nu\rangle\Big)^2 \Big/ \Big(\sum_\nu \frac{e^{-\beta E_\nu}}{Z}\delta E_\nu^2\Big) \geq 0 \tag{S12}$$

from the Cauchy-Schwarz inequality. Here $\langle\nu'|\hat{m}^0_{\boldsymbol{k}=\mathbf{0}}|\nu\rangle = \delta_{\nu,\nu'}\langle\nu|\hat{m}^0_{\boldsymbol{k}=\mathbf{0}}|\nu\rangle = \delta_{\nu,\nu'}\langle\nu|\hat{\sigma}^z_{\mathbf{0}}|\nu\rangle$ holds, since $|\nu\rangle$ is the simultaneous eigenstate of $\hat{H}(h)$, translation operators, and $\hat{m}^0_{\boldsymbol{k}=\mathbf{0}}$. This yields the general relation (7) [2–4]. The equality for finite $N$ holds if and only if $\langle\nu|\hat{\sigma}^z_{\mathbf{0}}|\nu\rangle = C\ \delta E_\nu/N$ for all $\nu$, where $C$ is some constant independent of $\nu$. This is not satisfied in almost all systems. In the thermodynamic limit $N\to\infty$, the condition for the equality is relaxed as follows.

Result (i) : From Eq. (S12), the necessary and sufficient condition for Eq. (4) is given as

$$\lim_{N\to\infty}\sum_\nu \frac{e^{-\beta E_\nu}}{Z} N\Big|\langle\nu|\delta\hat{\sigma}^z_{\mathbf{0}}|\nu\rangle - \big(\textstyle\sum_{\nu'}\frac{e^{-\beta E_{\nu'}}}{Z}\delta E_{\nu'}\langle\nu'|\delta\hat{\sigma}^z_{\mathbf{0}}|\nu'\rangle\big)\delta E_\nu \Big/ \big(\textstyle\sum_{\nu'}\frac{e^{-\beta E_{\nu'}}}{Z}\delta E_{\nu'}^2\big)\Big|^2 = 0. \tag{S13}$$

This condition can be rephrased as Eq. (8), where the constant $C$ is given by

$$C = N\big(\textstyle\sum_{\nu'}\frac{e^{-\beta E_{\nu'}}}{Z}\delta E_{\nu'}\langle\nu'|\delta\hat{\sigma}^z_{\mathbf{0}}|\nu'\rangle\big) \Big/ \big(\textstyle\sum_{\nu'}\frac{e^{-\beta E_{\nu'}}}{Z}\delta E_{\nu'}^2\big) + o(1), \tag{S14}$$

which does not vanish in our case for the reasons explained below Eq. (2) of the main text.

We can relate condition (8) with the ordinary ETH more directly. Let us introduce the microcanonical average over the energy shell $(E-\delta, E]$ as $\langle\bullet\rangle_{\rm mc}(E/N)$ and the number of states in $(E-\delta,E]$ as $W(E/N)$, assuming that the energy width $\delta$ can be taken as $\delta_N = \Theta(1/N^{1+\alpha})$, where $\alpha$ is some small positive number. Then we can evaluate $\langle\hat{\sigma}^z_{\mathbf{0}}\rangle_{\rm ini}$ as

$$\langle\hat{\sigma}^z_{\mathbf{0}}\rangle_{\rm ini} = \sum_\nu \frac{e^{-\beta E_\nu}}{Z}\langle\nu|\hat{\sigma}^z_{\mathbf{0}}|\nu\rangle = \frac{\int {\rm d}e \exp(N(s_N(e)-\beta e))\langle\hat{\sigma}^z_{\mathbf{0}}\rangle_{\rm mc}(e)}{\int {\rm d}e\exp(N(s_N(e)-\beta e))} + \mathcal{O}(\delta_N), \tag{S15}$$

where $s_N(e) = \log W(e)/N$. Except at a phase transition point, we can use the saddle point method and obtain

$$\langle\hat{\sigma}^z_{\mathbf{0}}\rangle_{\rm ini} = \langle\hat{\sigma}^z_{\mathbf{0}}\rangle_{\rm mc}(e^*) + \mathcal{O}(1/N), \tag{S16}$$

where $e^*$ is determined by $s_N'(e^*) = \frac{{\rm d}s_N}{{\rm d}e}(e^*) = \beta$. In the same way,

$$\langle\hat{H}(h)\rangle_{\rm ini}/N = e^* + \mathcal{O}(1/N), \tag{S17}$$

$$\sum_\nu \frac{e^{-\beta E_\nu}}{Z}\delta E_\nu^2 \Big/ N = 1/|s_N''(e^*)| + o(1), \tag{S18}$$

$$\sum_\nu \frac{e^{-\beta E_\nu}}{Z}\delta E_\nu\langle\nu|\delta\hat{\sigma}^z_{\mathbf{0}}|\nu\rangle = \frac{{\rm d}\langle\hat{\sigma}^z_{\mathbf{0}}\rangle_{\rm mc}}{{\rm d}e}(e^*) \Big/ |s_N''(e^*)| + o(1), \tag{S19}$$

$$N\sum_\nu \frac{e^{-\beta E_\nu}}{Z}\langle\nu|\delta\hat{\sigma}^z_{\mathbf{0}}|\nu\rangle^2 = N\sum_\nu\frac{e^{-\beta E_\nu}}{Z}|\langle\nu|\hat{\sigma}^z_{\mathbf{0}}|\nu\rangle - \langle\hat{\sigma}^z_{\mathbf{0}}\rangle_{\rm mc}(E_\nu/N)|^2 + \Big(\frac{{\rm d}\langle\hat{\sigma}^z_{\mathbf{0}}\rangle_{\rm mc}}{{\rm d}e}(e^*)\Big)^2 \Big/ |s_N''(e^*)| + o(1) \tag{S20}$$

can be shown. From Eqs. (S18), (S19), and (S20), the following result holds.

Result (i') : Eq. (4) or its equivalent condition (8) holds if and only if

$$N\sum_\nu\frac{e^{-\beta E_\nu}}{Z}|\langle\nu|\hat{\sigma}^z_{\mathbf{0}}|\nu\rangle - \langle\hat{\sigma}^z_{\mathbf{0}}\rangle_{\rm mc}(E_\nu/N)|^2 = o(1), \tag{S21}$$

which is similar to the weak ETH [5–7] in that it requires almost all $\langle\nu|\hat{\sigma}^z_{\mathbf{0}}|\nu\rangle$ should be close to $\langle\hat{\sigma}^z_{\mathbf{0}}\rangle_{\rm mc}(E_\nu/N)$. Condition (S21) will be satisfied in nonintegrable systems, where $\langle\nu|\hat{\sigma}^z_{\mathbf{0}}|\nu\rangle$ is often exponentially close to $\langle\hat{\sigma}^z_{\mathbf{0}}\rangle_{\rm mc}(E_\nu/N)$ [8, 9]. Note that, there are some integrable models which satisfy the ordinary weak ETH [5, 6, 10] but do not satisfy condition (S21). This fact can be confirmed by the violation of its equivalent Eq. (4), $\chi_\infty^{\rm qch}(\mathbf{0}) = \chi_\infty^S(\mathbf{0})$. (See main text.) Indeed, condition (S21) is more stringent than the ordinary weak ETH [5, 6, 10] in that condition (S21) requires

$|\langle\nu|\hat{\sigma}^z_{\mathbf{0}}|\nu\rangle - \langle\hat{\sigma}^z_{\mathbf{0}}\rangle_{\mathrm{mc}}(E_\nu/N)|^2$ to be typically $o(1/N)$, while the ordinary weak ETH [5, 6, 10] allows this quantity to be larger than $\Theta(1/N)$. Here, functions of $N$, $f_N$ and $g_N$, satisfy $g_N = \Theta(f_N)$, if there are positive constants $0 < c_1 \le c_2 < \infty$ such that $c_1 f_N \le g_N \le c_2 f_N$ holds for sufficiently large $N$.

Eqs. (S3) and (S5) give a relation between $\boldsymbol{k} \neq \mathbf{0}$ components,

$$\chi^T_N(\boldsymbol{k}) - \chi^{\mathrm{qch}}_N(\boldsymbol{k}) = \beta N\langle\delta\hat{m}^0_{\boldsymbol{k}};\delta\hat{m}^0_{\boldsymbol{k}}\rangle = \beta N\sum_\nu \frac{e^{-\beta E_\nu}}{Z}\sum_{\nu'}\delta_{E_\nu,E_{\nu'}}\delta_{\boldsymbol{K}_\nu,\boldsymbol{K}_{\nu'}+\boldsymbol{k}}|\langle\nu'|\hat{\sigma}^z_{\mathbf{0}}|\nu\rangle|^2, \tag{S22}$$

where the crystal momentum $\boldsymbol{K}_\nu$ is defined so that the eigenvalue of $\boldsymbol{r}$ sites translation operator is written as $e^{-i\boldsymbol{K}_\nu\cdot\boldsymbol{r}}$ and we used $|\langle\nu'|\hat{m}_{\boldsymbol{k}}|\nu\rangle| = \delta_{\boldsymbol{K}_\nu,\boldsymbol{K}_{\nu'}+\boldsymbol{k}}|\langle\nu'|\hat{\sigma}^z_{\mathbf{0}}|\nu\rangle|$. Therefore Eqs. (S10) and (S22) yield the following.

Result (ii) : Eq. (5) holds if and only if the off-diagonal elements are small so that

$$\sum_\nu \frac{e^{-\beta E_\nu}}{Z} N\sum_{\nu'}\delta_{E_\nu,E_{\nu'}}\delta_{\boldsymbol{K}_\nu,\boldsymbol{K}_{\nu'}+\boldsymbol{k}}|\langle\nu'|\hat{\sigma}^z_{\mathbf{0}}|\nu\rangle|^2 = o(1) \quad \text{for all } \boldsymbol{k}\neq\mathbf{0}. \tag{S23}$$

This condition can be rephrased as Eq. (10), which is weaker than the ordinary off-diagonal ETH [11–14] as explained below using $XY$ model.

### D. Analysis of the quench process using thermodynamics

In this section, we assume that thermalization occurs after the quench process, where the small uniform magnetic field $\Delta h_{\mathbf{0}}$ is applied. From this assumption, the state of the system, which evolves from the initial equilibrium state, relaxes to another equilibrium state. Since the expectation value of the postquench Hamiltonian $\hat{H}(h+\Delta h_{\mathbf{0}})$ does not change before and after the quench, the initial and the final equilibrium states satisfy

$$e+\Delta e = \langle\hat{H}(h+\Delta h_{\mathbf{0}})\rangle_{\mathrm{fin}}/N = \langle\hat{H}(h+\Delta h_{\mathbf{0}})\rangle_{\mathrm{ini}}/N = \langle\hat{H}(h)\rangle_{\mathrm{ini}}/N - \langle\hat{m}_{\mathbf{0}}\rangle_{\mathrm{ini}}\Delta h_{\mathbf{0}} = e - m_{\mathbf{0}}\Delta h_{\mathbf{0}}, \tag{S24}$$

where $e$ and $e+\Delta e$ are the initial and the final equilibrium values of the energy per site and $m_{\mathbf{0}}$ is the initial equilibrium value of the $\boldsymbol{k}=\mathbf{0}$ component of the magnetization. From Eq. (S24), the change of the entropy is

$$\Delta s = \frac{\partial s}{\partial e}(e,h)\Delta e + \frac{\partial s}{\partial h}(e,h)\Delta h_{\mathbf{0}} + \mathcal{O}\big((\Delta h_{\mathbf{0}})^2\big) = \beta\Delta e + \beta m_{\mathbf{0}}\Delta h_{\mathbf{0}} + \mathcal{O}\big((\Delta h_{\mathbf{0}})^2\big) = \mathcal{O}\big((\Delta h_{\mathbf{0}})^2\big), \tag{S25}$$

where $\beta$ is the initial inverse temperature. Eq. (S25) is consistent with Eq. (4). Note that the change of the energy per site $\Delta e = -m_{\mathbf{0}}\Delta h_{\mathbf{0}}$ and the change of the inverse temperature

$$\Delta\beta = \frac{\beta}{c_h}\Big(\frac{\partial m_{\mathbf{0}}}{\partial T}\Big)_h\Delta h_{\mathbf{0}} + \mathcal{O}\big((\Delta h_{\mathbf{0}})^2\big) \tag{S26}$$

are $\mathcal{O}(\Delta h_{\mathbf{0}})$ because $h\neq 0$. This results in $\chi^{\mathrm{qch}}_\infty(\mathbf{0}) < \chi^T_\infty(\mathbf{0})$.

### E. Proof of (iii)

From condition (12), we can define $\chi^{\mathrm{inf}}(\boldsymbol{k}) = \lim_{N\to\infty}\sum_{\boldsymbol{r}\in\Omega_N} e^{-i\boldsymbol{k}\cdot\boldsymbol{r}}\phi^T_\infty(\boldsymbol{r})$, which is uniformly continuous in $\boldsymbol{k}$ by the property of Fourier transform. From Eq. (S5),

$$|\chi^T_N(\boldsymbol{k}) - \chi^{\mathrm{inf}}(\boldsymbol{k})| \le \Big|\sum_{\boldsymbol{r}\in\Omega_N} e^{-i\boldsymbol{k}\cdot\boldsymbol{r}}\big(\phi^T_N(\boldsymbol{r}) - \phi^T_\infty(\boldsymbol{r})\big)\Big| + \Big|\lim_{N'\to\infty}\sum_{\boldsymbol{r}\in\Omega_{N'}\setminus\Omega_N} e^{-i\boldsymbol{k}\cdot\boldsymbol{r}}\phi^T_\infty(\boldsymbol{r})\Big| \tag{S27}$$

$$\le \sum_{\boldsymbol{r}\in\Omega_N}\big|\phi^T_N(\boldsymbol{r}) - \phi^T_\infty(\boldsymbol{r})\big| + \lim_{N'\to\infty}\sum_{\boldsymbol{r}\in\Omega_{N'}\setminus\Omega_N}\big|\phi^T_\infty(\boldsymbol{r})\big|. \tag{S28}$$

In the $N\to\infty$ limit, the first term and the second term of Eq. (S28) converges to 0 from condition (13) and (12), respectively. As a result, $\chi^T_N(\boldsymbol{k})$ converges to $\chi^{\mathrm{inf}}(\boldsymbol{k})$ in the $N\to\infty$ limit, $\chi^T_\infty(\boldsymbol{k}) = \chi^{\mathrm{inf}}(\boldsymbol{k})$ for all $\boldsymbol{k}$, which implies that $\chi^T_\infty(\boldsymbol{k})$ is also uniformly continuous in $\boldsymbol{k}$. □

Note that condition (13) is essential for the uniform continuity of $\chi^T_\infty(\boldsymbol{k})$. Since $\phi^S_\infty(\boldsymbol{r}) = \phi^T_\infty(\boldsymbol{r})$ for all $\boldsymbol{r}$ follows from Eq. (S8), condition (12) holds also for $\phi^S$. However condition (13) does not hold for $\phi^S$:

$$\lim_{N\to\infty}\sum_{\boldsymbol{r}\in\Omega_N}|\phi^S_N(\boldsymbol{r}) - \phi^S_\infty(\boldsymbol{r})| = \lim_{N\to\infty}\sum_{\boldsymbol{r}\in\Omega_N}|\phi^S_N(\boldsymbol{r}) - \phi^T_N(\boldsymbol{r}) + \phi^T_N(\boldsymbol{r}) - \phi^T_\infty(\boldsymbol{r})| = \chi^T_\infty(\mathbf{0}) - \chi^S_\infty(\mathbf{0}) > 0, \tag{S29}$$

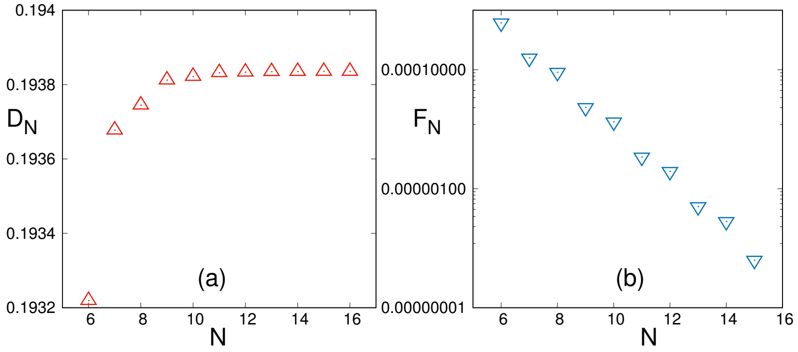


FIG. S2. Verification of conditions for (iii) in $XYZ$ model, with the same parameters as in Fig. S1. We investigate the $N$ dependence of (a)$D_N$, the sum of $|\phi^T_{N_{\max}}(\boldsymbol{r})|$ over all $\boldsymbol{r} \in \Omega_N$, and (b)$F_N$, the sum of $|\phi^T_N(\boldsymbol{r}) - \phi^T_{N_{\max}}(\boldsymbol{r})|$ over all $\boldsymbol{r} \in \Omega_N$. We take $N_{\max} = 16$.

which is consistent with the discontinuity of $\chi^S_\infty(\boldsymbol{k})$ at $\boldsymbol{k} = \boldsymbol{0}$.

In Fig. S2, we verify the conditions for (iii), (a) $\phi^T_\infty(\boldsymbol{r})$ decays fast enough and (b) finite-size effects of $\phi^T_N(\boldsymbol{r})$ are small, in $XYZ$ model. To this end, we introduce two quantities, (a)$D_N = \sum_{\boldsymbol{r}\in\Omega_N} |\phi^T_{N_{\max}}(\boldsymbol{r})|$ and (b)$F_N = \sum_{\boldsymbol{r}\in\Omega_N} |\phi^T_N(\boldsymbol{r}) - \phi^T_{N_{\max}}(\boldsymbol{r})|$, where $N_{\max}$ is taken as large as possible. Fig. S2 (a) shows $N$ dependence of $D_N$ in $XYZ$ model. As $N$ increases, $D_N$ is saturated, suggesting that condition (12) holds. Fig. S2 (b) shows $N$ dependence of $F_N$ in the same system. As $N$ increases, $F_N$ decreases, suggesting that condition (13) holds.

### F. Analytic solutions in 1D $XY$ model

We here describe the analytic solutions $\chi^{\rm qch}_\infty(k)$, $\chi^S_\infty(k)$, and $\chi^T_\infty(k)$ in 1D $XY$ model and verify whether the above relations hold or not in this model. By defining $J_s = J_x + J_y$, $J_a = J_x - J_y$, and $\varepsilon_k = \sqrt{(J_s \cos k + h)^2 + J_a^2 \sin^2 k}$, we can write the results as follows.

For the $k = 0$ components, we have

$$\chi^{\rm qch}_\infty(0) = \frac{1}{2\pi}\int_0^{2\pi} \mathrm{d}k' \, \frac{J_a^2 \sin^2 k'}{\varepsilon_{k'}^2} \frac{\tanh \beta\varepsilon_{k'}}{\varepsilon_{k'}}, \tag{S30}$$

$$\chi^T_\infty(0) = \chi^{\rm qch}_\infty(0) + \frac{\beta}{2\pi}\int_0^{2\pi} \mathrm{d}k' \, \frac{(J_s \cos k' + h)^2}{\varepsilon_{k'}^2} \frac{1}{\cosh^2 \beta\varepsilon_{k'}}, \tag{S31}$$

$$\chi^S_\infty(0) = \chi^T_\infty(0) - \left(\frac{\beta}{2\pi}\int_0^{2\pi} \mathrm{d}k' \, \frac{J_s \cos k' + h}{\cosh^2 \beta\varepsilon_{k'}}\right)^2 \Big/ \left(\frac{\beta}{2\pi}\int_0^{2\pi} \mathrm{d}k' \, \frac{\varepsilon_{k'}^2}{\cosh^2 \beta\varepsilon_{k'}}\right) < \chi^T_\infty(0). \tag{S32}$$

From Eqs. (S30) and (S32), Eq. (4) is violated except at $J_s = J_a = 0$ [free spin model] or $|J_s| = |J_a| = |h|$ [a special case of the transverse field Ising model]. Therefore, condition (8) does not hold, whereas the ordinary weak ETH [5, 6, 10] is satisfied in this model.

For the $k \neq 0$ components, Eq. (5) is satisfied as

$$\begin{aligned}
\chi^T_\infty(k) &= \chi^S_\infty(k) = \chi^{\rm qch}_\infty(k) \\
&= \frac{1}{2\pi}\int_0^{2\pi} \mathrm{d}k' \frac{\varepsilon_{k'}\varepsilon_{k'+k} - (J_s \cos k' + h)(J_s \cos(k'+k) + h) + J_a^2 \sin k' \sin(k'+k)}{2\varepsilon_{k'}\varepsilon_{k'+k}} \\
&\qquad \times \frac{\tanh \beta\varepsilon_{k'} + \tanh \beta\varepsilon_{k'+k}}{\varepsilon_{k'} + \varepsilon_{k'+k}} \\
&\quad + \frac{1}{2\pi}\int_0^{2\pi} \mathrm{d}k' \frac{\sinh \beta(\varepsilon_{k'} - \varepsilon_{k'+k})}{\varepsilon_{k'} - \varepsilon_{k'+k}} \frac{1}{\cosh \beta\varepsilon_{k'} \cosh \beta\varepsilon_{k'+k}} \\
&\qquad \times \frac{\varepsilon_{k'}\varepsilon_{k'+k} + (J_s \cos k' + h)(J_s \cos(k'+k) + h) - J_a^2 \sin k' \sin(k'+k)}{2\varepsilon_{k'}\varepsilon_{k'+k}}.
\end{aligned} \tag{S33}$$

This indicates condition (S23) is satisfied in this model. From Eqs. (S31) and (S33), Eq. (6) holds and $\chi^T_\infty(k)$ is uniformly continuous in $k$, while $\chi^{\rm qch}_\infty(k)$ is discontinuous at $k=0$. Moreover, for $k\neq 0$, $\chi^T_N(k)-\chi^{\rm qch}_N(k)$ scales as

$$\chi^T_N(k)-\chi^{\rm qch}_N(k)=\frac{\beta}{2N}\left(\frac{1}{\cosh^2\beta\varepsilon_{k/2}}+\frac{1}{\cosh^2\beta\varepsilon_{\pi-k/2}}\right)+\exp\bigl(-\Theta(N)\bigr)=\Theta(1/N), \tag{S34}$$

because some off-diagonal elements $|\langle\nu'|\hat{\sigma}^z_j|\nu\rangle|$ that are appeared in Eq. (S23) scale as $\Theta(1/N)$. That indicates the ordinary off-diagonal ETH [11–14], which requires exponentially fast decay of all off-diagonal elements, is not satisfied in this model.

### G. Additional demonstrations of (ii)-(iv)

Although condition (S23) is weaker than the ordinary off-diagonal ETH [11–14] as mentioned above, there are some models which do not satisfy it such as the longitudinal field Ising model ($J_x=J_y=0$). Fig. S3 (a) shows $k$ dependence of $\chi^{\rm qch}_N(k)$, $\chi^T_N(k)$, and $\chi^S_N(k)$ in this model. Since $\hat{m}_k$ is conserved, $\chi^{\rm qch}_N(k)=0$ holds, while $\chi^T_N(k)$ and $\chi^S_N(k)>0$ for all $k$, resulting in the violation of Eq. (5) or equivalent condition (S23). In contrast, Fig. S3 (b) shows how the susceptibilities behave when a small nonintegrability ($J_x+J_y=0.1$, $J_x-J_y=0.2$) is added to this system. For the $k=0$ component, $\chi^{\rm qch}_N(0)$ does not approach $\chi^S_N(0)$ as $N$ is increased, and Eq. (4) is not satisfied as in (a). On the other hand, the $k\neq 0$ components $\chi^{\rm qch}_N(k)$ differs dramatically from those of (a), and Eq. (5) seems satisfied in (b).

These results suggest that Eq. (5) is easily satisfied as in (b), while we need more nonintegrability for Eq. (4). Reflecting these facts, $\chi^{\rm qch}_\infty(k)$ is discontinuous at $k=0$ in only (b), while $\chi^T_\infty(k)$ is uniformly continuous in both (a) and (b).

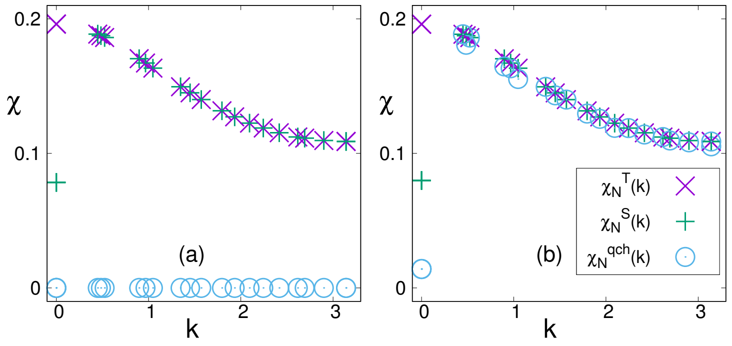


FIG. S3. $k$ dependence of $\chi^{\rm qch}_N(k)$, $\chi^T_N(k)$, and $\chi^S_N(k)$ in (a) longitudinal field Ising model ($J_x=J_y=0$) and (b) $XYZ$ model with small $J_x$ and $J_y$ ($J_x+J_y=0.1$, $J_x-J_y=0.2$). $J_z=1.0$, $h=0.8$, and $\beta=0.15$ are fixed. We take $N=$ 12-14 and $k=2\pi n_k/N$ with $n_k\in\mathbb{Z}$.

### H. Relation to Kubo formula

The susceptibility obtained by Kubo formula [15, 16] is given as

$$\chi^{\rm Kubo}_N(\boldsymbol{k},\omega+i\varepsilon)=\int_0^\infty {\rm d}t\, e^{i\omega t-\varepsilon t}\frac{N}{i}\langle[\hat{m}_{\boldsymbol{k}}(t),-\hat{m}^\dagger_{\boldsymbol{k}}]\rangle_{\rm ini} \tag{S35}$$

$$=\chi^T_N(\boldsymbol{k})+(i\omega-\varepsilon)\int_0^\infty {\rm d}t\, e^{i\omega t-\varepsilon t}\beta N\langle\delta\hat{m}_{\boldsymbol{k}};\delta\hat{m}_{\boldsymbol{k}}(t)\rangle_{\rm ini}, \tag{S36}$$

where $[\hat{X},\hat{Y}]=\hat{X}\hat{Y}-\hat{Y}\hat{X}$ is the commutator, $\omega$ is the angular frequency, and $\varepsilon$ is a small positive number.

From Eqs. (S36) and (S3), the following holds for all $N$ and for all $\boldsymbol{k}$,

$$\lim_{\varepsilon\to+0}\chi^{\rm Kubo}_N(\boldsymbol{k},0+i\varepsilon)=\chi^T_N(\boldsymbol{k})-\beta N\langle\delta\hat{m}^0_{\boldsymbol{k}};\delta\hat{m}^0_{\boldsymbol{k}}\rangle_{\rm ini}=\chi^{\rm qch}_N(\boldsymbol{k}). \tag{S37}$$

[1] S. Trotzky, Y. A. Chen, A. Flesch, I. P. McCulloch, U. Schollwöck, J. Eisert, and I. Bloch, Probing the relaxation towards equilibrium in an isolated strongly correlated one-dimensional Bose gas, Nat. Phys. **8**, 325 (2012).
[2] R. M. Wilcox, Bounds for the Isothermal, Adiabatic, and Isolated Static Susceptibility Tensors, Phys. Rev. **174**, 624 (1968).
[3] P. Mazur, Non-ergodicity of phase functions in certain systems, Physica **43**, 533 (1969).
[4] M. Suzuki, Ergodicity, constants of motion, and bounds for susceptibilities, Physica **51**, 277 (1971).
[5] G. Biroli, C. Kollath, and A. M. Läuchli, Effect of Rare Fluctuations on the Thermalization of Isolated Quantum Systems, Phys. Rev. Lett. **105**, 250401 (2010).
[6] E. Iyoda, K. Kaneko, and T. Sagawa, Fluctuation Theorem for Many-Body Pure Quantum States, Phys. Rev. Lett. **119**, 100601 (2017).
[7] T. Mori, Weak eigenstate thermalization with large deviation bound, arXiv:1609.09776.
[8] W. Beugeling, R. Moessner, and M. Haque, Finite-size scaling of eigenstate thermalization, Phys. Rev. E **89**, 042112 (2014).
[9] R. Steinigeweg, A. Khodja, H. Niemeyer, C. Gogolin, and J. Gemmer, Pushing the Limits of the Eigenstate Thermalization Hypothesis towards Mesoscopic Quantum Systems, Phys. Rev. Lett. **112**, 130403 (2014).
[10] T. Kuwahara and K. Saito, Ensemble equivalence and eigenstate thermalization from clustering of correlation, arXiv:1905.01886.
[11] M. Srednicki, The approach to thermal equilibrium in quantized chaotic systems, J. Phys. A **32**, 1163 (1999).
[12] L. D'Alessio, Y. Kafri, A. Polkovnikov, and M. Rigol, From quantum chaos and eigenstate thermalization to statistical mechanics and thermodynamics, Adv. Phys. **65**, 239 (2016).
[13] T. Mori, T. N. Ikeda, E. Kaminishi, and M. Ueda, Thermalization and prethermalization in isolated quantum systems: a theoretical overview, J. Phys. B **51**, 112001 (2018).
[14] F. Anza, C. Gogolin, and M. Huber, Eigenstate Thermalization for Degenerate Observables, Phys. Rev. Lett. **120**, 150603 (2018).
[15] R. Kubo, Statistical-Mechanical Theory of Irreversible Processes. I. General Theory and Simple Applications to Magnetic and Conduction Problems, J. Phys. Soc. Jpn. **12**, 570 (1957).
[16] R. Kubo, M. Toda, and N. Hashitsume, *Statistical Physics II*, 2nd ed. (Springer, Berlin, 1991).
